# Supplementary material for: Understanding and Improving the Latency of DRAM-Based Memory Systems
Source: arXiv:1712.08304 source file (2017-12-22)
Supplement: Supplementary file 1 [file appendix.tex]

%\vspace{-0.5in}
\appendix
\label{sec:appendix}

%\section{Characterization Tests}
%\subsection{Activation Error Analysis}
%\label{app_rcd_test}
%\input{sec/algos/trcdlocal}

%\vspace{0.2in}
%\subsection{Precharge Latency Variation} %(\secref{trp_tests})}
%\label{app_rp_test}
%\input{sec/algos/trptest}

%%%%%%%%%%%

%\section{Analysis on Activation Latency}

%\subsection{Bank to Bank Variation}
%\label{app_bank}
%%\noindent\textbf{Activation Errors: Bank to Bank Variation (\secref{trcd_loc}).}
%
%\figref{dimm_y17_rcd3} shows the distribution of
%activation errors in every bank of \dimm{0}{C}, observed from 52 experimental
%test rounds. Some banks experience more errors than others, demonstrating
%non-uniform distribution of activation errors.

%%%%%%%%%%%

%\noindent\textbf{Distribution of Errors in Data Bursts (\secref{density_err}).}
%\subsection{Distribution of Errors in Data Bursts}

%\section{Distribution of Activation Errors in Data Beats}
\section{Activation Errors in Data Beats}
\label{app_err_bursts}

\figref{burst_rcd2_20c} shows the distribution of \newt{bit error} observed in each
data beat of all erroneous cache lines when using \trcde5ns. We show experiments
from 9 DIMMs, categorized into three DIMM models (one per vendor). Compared to
using \trcde7.5ns (\figref{burst_rcd3_20c}), the number of bit errors increases
in every beat. However, for some DIMMs, the number of beats without errors is
still significantly high.

\begin{figure}[!h]
    \centering
    \captionsetup[subfigure]{justification=centering}
    %\subcaptionbox{Two DIMMs (A-M1).}[0.3\textwidth]
    %{
    %    \includegraphics[width=0.3\linewidth]{plots/trcd/bursts/all_cr_m1_dimms_burst_rcd2.pdf}
    %}
    %%
    %\subcaptionbox{One DIMMs (B-M1).}[0.3\textwidth]
    %{
    %    \includegraphics[width=0.3\linewidth]{plots/trcd/bursts/all_hy_m1_dimms_burst_rcd2.pdf}

    %}
    %%
    %\subcaptionbox{Six DIMMs (C-M0).}[0.3\textwidth]
    %{
    %    \includegraphics[width=0.3\linewidth]{plots/trcd/bursts/all_y_dimms_burst_rcd2.pdf}
    %}

    \subcaptionbox{A-M1}%[\linewidth]
    {
        \includegraphics[width=0.46\linewidth]{plots/trcd/bursts/all_cr_m1_dimms_burst_rcd2.pdf}
        \vspace{-5pt}
    }
    \subcaptionbox{B-M1}%[\linewidth]
    {
        \includegraphics[width=0.46\linewidth]{plots/trcd/bursts/all_hy_m1_dimms_burst_rcd2.pdf}
        \vspace{-5pt}
    }
    \subcaptionbox{C-M0}[\linewidth]
    {
        \includegraphics[width=0.46\linewidth]{plots/trcd/bursts/all_y_dimms_burst_rcd2.pdf}
        \vspace{-5pt}
    }

    \caption{Breakdown of the number of error bits observed in each data
    beat of erroneous cache lines at \trcde5ns.}
    \label{fig:burst_rcd2_20c}
\end{figure}

%all_cr_m1_dimms_burst_rcd2.pdf
%all_hy_m1_dimms_burst_rcd2.pdf
%all_y_dimms_burst_rcd2.pdf

%\begin{figure*}[h]
%    \centering
%    \captionsetup[subfigure]{justification=centering}
%    \subcaptionbox{DIMM A0.}[0.225\textwidth]
%    {
%        \includegraphics[width=0.225\linewidth]{plots/trcd/bursts/b1_all_patt_rcd2_20c.pdf}
%    }
%    %
%    \subcaptionbox{DIMM B0.}[0.225\textwidth]
%    {
%        \includegraphics[width=0.225\linewidth]{plots/trcd/bursts/burst_dist_p6_all_att_rcd2.pdf}
%    }
%    %
%    \subcaptionbox{DIMM C0.}[0.225\textwidth]
%    {
%        \includegraphics[width=0.225\linewidth]{plots/trcd/bursts/burst_dist_y22_all_patt_rcd2_20c.pdf}
%    }
%    %
%    \subcaptionbox{DIMM C5.}[0.225\textwidth]
%    {
%        \includegraphics[width=0.225\linewidth]{plots/trcd/bursts/burst_dist_g1_all_patt_rcd2_20c.pdf}
%    }
%
%    \caption{Breakdown on the number of error bits observed in data
%    bursts, which form a cache line, due to \trcd=5ns at 20\celsius.}
%    \label{fig:burst_rcd2_20c}
%\end{figure*}

%%%%%%%%%%%

%\newpage

%%%%%%%%%%%

\ignore{
\section{Exploiting Latency Variation: Column Command Re-Ordering}
%\label{sec:col_comm_reorder}
\label{app_col_comm_reorder}

As we observed in Section~\ref{sec:trcd_errors:first_col}, when the activation
latency is lowered aggressively, errors can appear when reading from DRAM, but
\emph{only} within the first cache line that is read out.  We also observed in
Section~\ref{sec:trcd_loc} that these errors do not occur uniformly across a
DIMM, and that errors tend to cluster within only certain columns of a row.
Based on these observations, we develop a scheduling mechanism whose
goal is to reduce the probability of errors due to shortened activation latency,
by reordering requests such that the first column accessed is the most robust.

When a row is activated, there is often more than one request to access that
row, due to spatial locality.  Several memory scheduling algorithms, such as
the widely-used FR-FCFS\ignore{~\cite{rixner-isca2000}}, work to exploit \emph{row buffer
locality}, where multiple pending requests to an activated row are sent
back-to-back in order to avoid activating the row multiple times (and incurring
additional activation and precharge latencies).  To do this, memory schedulers
reorder the pending requests to DRAM by adding a set of prioritization
rules. %(e.g.,~\cite{rixner-isca2000,mutlu-isca2008,kim-micro2010,subramanian-iccd2014}).

We propose a memory scheduler where we expose the reliability of each column
within a row.  Similar to our approach in Section~\ref{sec:var_latency_mc}, we
perform profiling to classify the expected number of errors for each cache line
within a row, and store this within a table in the memory controller.  We then
feed this information into a modified version of the FR-FCFS scheduler, which
prioritizes pending requests to activated rows.  Our modified scheduler adds
another layer of prioritization amongst all of the pending requests to activated
rows, choosing the request whose desired cache line has the lowest expected
number of errors first.  When a requests first arrives into the memory
controller, the profiling data is looked up from the table, and then stored
alongside the other request data in the transaction queue.  The scheduler uses
the data in the transaction queue to make its decisions.

By reordering the requests, we expect that our scheduler can often find column
commands with no or very few errors, as we see many of these in
Section~\ref{sec:density_err}. Therefore, we conclude that a memory scheduler
that is aware of the distribution of errors across the cache lines within a row
can mitigate a large percentage of the errors that take place due to reduced
activation latency.
}
