# Supplementary material for: Understanding and Improving the Latency of DRAM-Based Memory Systems
Source: arXiv:1712.08304 source file (2017-12-22)
Supplement: Supplementary file 2 [file appendix.tex]

\appendix
\appendixpage

%\section{Bulk Copy Latency}
%\label{sec:appendix}

\vspace{-0.15in}
The bulk copy latencies reported in \tabref{copy_latency} are derived from the equations shown below.
%The energy numbers are reported by using the Micron power calculator~\cite{micron-tr}.

{
\setlength{\belowdisplayskip}{-4pt} \setlength{\belowdisplayshortskip}{0pt}
\setlength{\abovedisplayskip}{0pt} \setlength{\abovedisplayshortskip}{0pt}
\scriptsize
\vspace{-0.15in}
\begin{align}
\label{eq:1}
T_{memcpy} &= ((N_{col}-1)\times\tccd + \trp)\times2 + \trcd + \\
             &\phantom{{}=} \tcl + \tcwl + \trtw + \twr +\tbl \notag \\
\label{eq:2}
T_{\rcirsa} &= (\trcd + (N_{col}-1)\times\tccd + \trp)\times2 + \\
            & \phantom{{}=} \tcl + \tcwl + \twr \notag\\
\label{eq:3}
T_{\rcirba} &= \trcd + (N_{col}-1)\times\tccd + \tcl +\\
            &\phantom{{}=} \tcwl + \twr  + \trp  \notag\\
\label{eq:4}
T_{\rciasa} &= \tras\times2 + \trp \\
\label{eq:5}
T_{\lisarc} &= ACT_{src} + (RBM\times\ceil{\frac{hops}{2}} + PRE + \\
            & \phantom{{}=} ACT_{dst})\times2 \notag \\
            &= \tras + (RBM\times\ceil{\frac{hops}{2}} + \trp + \tras)\times2,
            \notag \\
            &where~RBM = 8ns~(\secref{lisa:variation}) \notag
\end{align}
\vspace{-0.15in}
}

In Eq.\eqref{eq:5}, we conservatively assume a one-hop RBM incurs the same
latency as a two-hop RBM. Hence the ceiling function on the hop counts.
